# Supplementary material for: Can one predict a drop contact angle?
Source: arXiv:2109.11040 ancillary file (2021-09-22)
Supplement: Supplementary file 1 [file Supplementary_Information.pdf]

# Supplementary Information for: Can one predict a drop contact angle?

Marion Silvestrini[*,1,2], Antonio Tinti[2], Alberto Giacomello[2], Carolina Brito[1]

[1]*Instituto de Física, Universidade Federal do Rio Grande do Sul, Av. Bento Gonçalves 9500, CEP 91501-970, Porto Alegre, Brazil*
[2]*Dipartimento di Ingegneria Meccanica e Aerospaziale, Università di Roma "La Sapienza", 00184 Rome, Italy*

September 22, 2021

In this supporting information it is described an algorithm to find the numerical solutions of a homogenised model and then the numerical solutions are compared with the free energy obtained with the simulations. We also present the criteria to adjust parameter $\kappa$, the error estimate of the free energy profile and description of the videos available. Finally the areas of the components for the proposed analytical free energy are presented.

## Numerical solution of the homogenised model

In the main text, we have introduced a model which takes into account the energy of creating interfaces of a 3D droplet with fixed volume $V_0 = 4/3\pi R_0^3$ when it is placed on a textured substrate. The droplet is allowed to display two wetting states, refereed as *ideal CB* and *ideal W*. For completeness, we rewrite the expressions for the difference in energy of a system with and without the droplet on the surface in both states:

$$\Delta E^{\mathbf{CB^I}} = \sigma_{\mathrm{GL}} \left[ S_{\mathrm{CB}} - \pi B_{\mathrm{CB}}^2 \left( \phi_{\mathrm{S}} \cos\theta_{\mathrm{Y}} - (1-\phi_{\mathrm{S}}) \right) \right], \quad (1)$$

$$\Delta E^{\mathbf{W^I}} = \sigma_{\mathrm{GL}} \left[ S_{\mathrm{W}} - \pi B_{\mathrm{W}}^2 \, r \cos\theta_{\mathrm{Y}} \right], \quad (2)$$

where $S_{\mathrm{s}} = 2\pi R^{\mathrm{s}2} \left[1 - \cos(\theta_{\mathrm{C}}^{\mathrm{s}})\right]$ is the surface of the spherical cap in contact with air, $B^{\mathrm{s}} = R^{\mathrm{s}} \sin(\theta_{\mathrm{C}}^{\mathrm{s}})$ is the base radius, $R^{\mathrm{s}}$ the radius of the droplet, and $\theta_{\mathrm{C}}^{\mathrm{s}}$ its contact angle in the state *s*. $\phi_{\mathrm{S}} = \mathrm{w}^2/\mathrm{d}^2$ is the fraction of solid surface area wet by the liquid (or pillar density) and $r = 1 + 4\mathrm{wh}/\mathrm{d}^2$ is the surface roughness ratio.

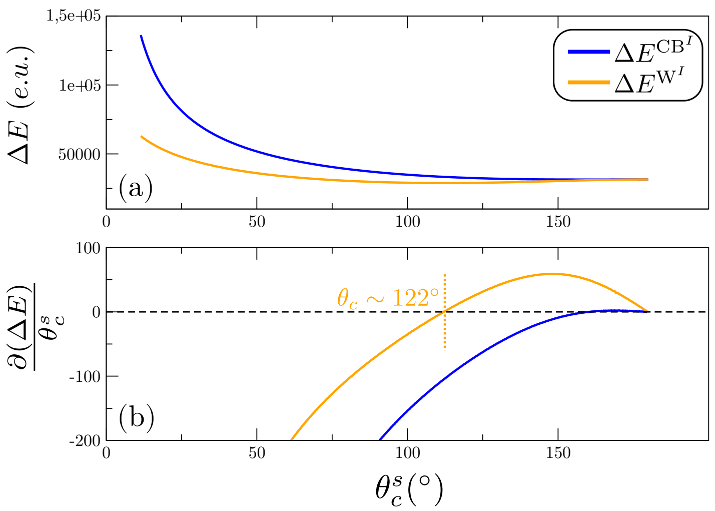


Figure 1: **(a)** $\Delta E^{\mathrm{CB^I}}$ in blue and $\Delta E^{\mathrm{W^I}}$ in orange, as a function of contact angle $\theta_c^s$. **(b)** Derivative of the energies as a function of $\theta_c^s$. $\theta_{\mathrm{C}} = 122°$ corresponds to the contact angle of the $W^I$ state, which is the wetting state that minimizes the energy of the droplet in this example.

To identify the stable wetting state $s$ between $\mathrm{W}^I$ and $\mathrm{CB}^I$, we minimize Equations (1) and (2) using an algorithm proposed previously [1, 2, 3] and outlined in the following. First, we fix the parameters of the surface $(\phi_{\mathrm{S}}, r, \theta_{\mathrm{Y}})$ and the droplet size $R_0$. Then, we vary $\theta_c^s$ to calculate the energies of the CB, $\Delta E^{\mathrm{CB^I}}$, and W state, $\Delta E^{\mathrm{W^I}}$ and find the minimum value of each one, $\Delta E^{\mathrm{CB}}_{\mathrm{min}}$ and $\Delta E^{\mathrm{W}}_{\mathrm{min}}$. Finally, we compare both minimum energy and find the lowest value to define the thermodynamic stable wetting state.

Figure (1)-a shows an example for a surface with parameters $(\phi_{\mathrm{S}} = 0.09, r = 1.78, \theta_{\mathrm{Y}} = 114°)$, which corresponds to a surface $\mathrm{S}_3$, on which a droplet of size $R_0 = 50$ is deposited. It is shown the numerical solution of $\Delta E^{\mathrm{CB^I}}$ in blue and $\Delta E^{\mathrm{W^I}}$ in orange as a function of $\theta_c^s$. It can be seen that $\Delta E^{\mathrm{W}}_{\mathrm{min}} < \Delta E^{\mathrm{CB}}_{\mathrm{min}}$, which indicates that W is the stable state. Then, by deriving the energy in relation to $\theta_c^s$, Figure (1)-b, we find the contact angle that minimizes that wetting state. For this surface, the droplet is in the W state with a contact angle given by $\theta_{\mathrm{C}} = 122°$.

# Simulation *vs* homogenised model

In Figure 2 we show a comparison between the numerical simulation and the homogeneous model. A sketch of $\mathrm{CB}^I$ and $\mathrm{W}^I$ is shown Figure 2-a. The green curve in panel **b** (for $\mathrm{S}_1$) and **c** (for $\mathrm{S}_3$) is the free energy from the MC simulation, $\Delta\mathcal{F}$, as a function of the *linear* cavities wetted. In orange we plot the the energy from Equation (1) and in purple is the energy from Equation (2)). In panel **d** we present the 3D visualization for the red triangle (maximum in $\Delta\mathcal{F}$) and black circle (global minimum in $\Delta\mathcal{F}$) highlighted in panel **c**. This is a view from below and the colors correspond to a pixel being filled by water or not. In this visualization we can see clearly the roughness of the area liquid-vapor, which is a key point for understanding the local minima discussed in the main text.

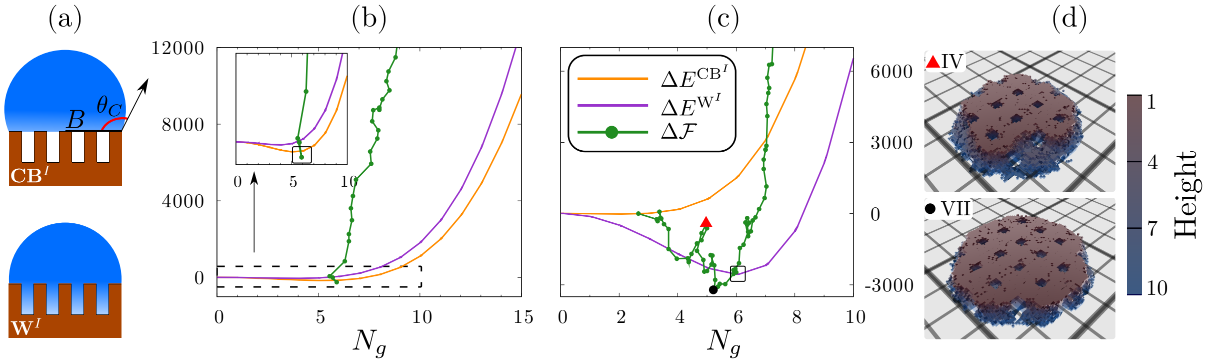


Figure 2: homogenised model *vs* $\Delta\mathcal{F}$. **(a)** Two types of configurations for the droplet considered in the homogenised model, CB$^I$ and W$^I$, with geometric definitions of the spherical droplet. **(b)** Numerical solution of Equations 1 and 2 compared to $\Delta\mathcal{F}$ for S$_1$. The inset in this figure is a zoom around the minimum value. **(c)** Same as in (b) for S$_3$. Energies are displaced by the same fixed value in $y$-axis to be able to compare with the variation of the free energy. Global minimum of the homogenised model is indicated by the open square. **(d)** Images of the 3D configurations of the droplet placed on S$_3$ for two values of fillings: in the maximum indicated by the red triangle in (c) and corresponding to the point IV in Figure 2-a and in the local minimum indicated by the black circle and corresponding to the point VII in Figure 2-a. This is a view from below and colors correspond to the filling of liquid in each pixel.

Figures 2-(b,c) show that there is a reasonable agreement between the continuous model and the simulation. For S$_1$ it is observed that $\Delta E^{\mathrm{CB^I}} < \Delta E^{\mathrm{W^I}}$, which means that the model predicts the droplet in the CB state. From $\Delta\mathcal{F}$ we see that the global minimum agrees with the prediction, the droplet is on the CB state on top of a similar value of pillars. For S$_3$ the picture is much more complex. The model predicts a drop on the Wenzel state wetting, although it cannot predict local minima, only the global one. On the other hand $\Delta\mathcal{F}$ does show many minima and, although they are not predicted, we observe that they are well aligned in the purple curve. For this surface the global minimum predicted and the one calculated does not agree quantitatively. An interesting point concerns the local minimum of CB.

Figures 2-(d) was shown in the main text and is presented here again to be contrasted with the ideal wetting states sketch in Figures 2-(a). In this last case, the W is supposed to homogeneously wet the surface, while the simulations shows a very rough interface between the liquid and the gas, which is not taken into account in the model. This important difference is one of the reasons why the model only predicts one global minimum for the W state while simulations finds several minima.

# Selecting numerical parameter

Before simulating the restrained Potts model we need to adjust the value of $\kappa$, the forcing parameter of the external bias in the Hamiltonian. In Figure 3 we show the filling $f$ as a function of $\kappa$ for the surface S$_3$. We select the first maxima (point II) in Figure 2 and run the simulation with the target value of this maxima and several values of $\kappa$. The black dashed line is the target value that we are imposing for the filling. In order to choose a correct value of $\kappa$ the initial condition cannot change the final configuration. So we tested two different initial conditions: CB$^0$ corresponds to a perfect sphere tangentially

touching the surface (purple curve), while $W^0$ is for a hemisphere (of same volume) wetting homogeneously the surface (orange curve).

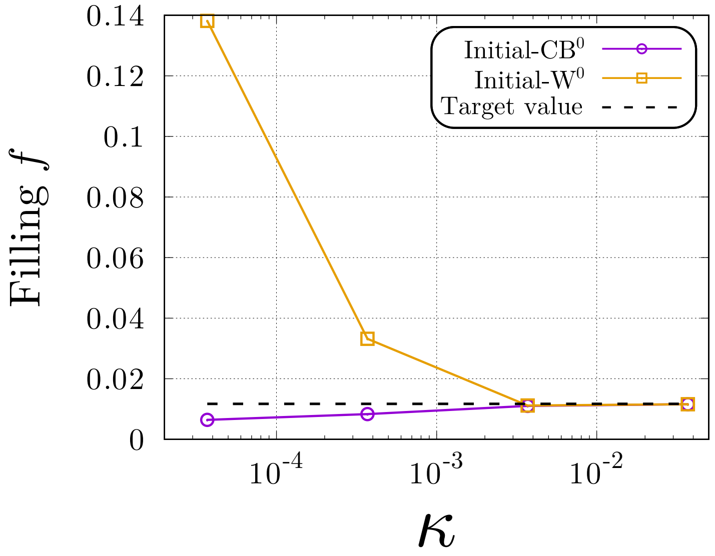


Figure 3: Filling $f$ as a function of the coupling parameter $\kappa$. Dashed black line is the target value of the maximum II from Figure 2. Orange curve correspond to a simulation with a hemisphere wetting the surface as initial condition (called $W^0$). The initial condition of the purple curve is a sphere touching the top of the pillar tangentially (called $CB^0$).

As expected, when we increase $\kappa$ the filling gets closer to its target value and the initial condition does not play a major role in the final configuration. In addition, it is also favorable to have some fluctuation in the system. Therefore, we select $\kappa = 0.004$, which is high enough that drives the system to the target configuration while allowing thermal fluctuations.

# 2D and 3D videos

The videos available show the free energy of each surface with a 2D or 3D representation of the droplet. In the 2D animation we show the side view of the droplet, while the 3D animation is a view from below and just showing the area liquid-vapor between the pillars. The black line is a guide to the eyes, showing the configuration in each point of the free energy.

# Interfacial areas

In the main text we proposed an analytical free energy written as

$$\Delta\Omega = \sigma_{\mathrm{GL}} \left( A^{\mathrm{C}}_{\mathrm{GL}} - \alpha V_0 + A^{\mathrm{B}}_{\mathrm{GL}} - A_{\mathrm{LS}} \cos\theta_{\mathrm{Y}} \right). \tag{3}$$

All the areas were calculated in the post processing part of the simulation. The spherical cap section of the gas-liquid interface, $A^{\mathrm{C}}_{\mathrm{GL}}$, and the bottom liquid-gas area, $A^{\mathrm{B}}_{\mathrm{GL}}$, have been divided by 1.5, which is a correcting factor for the increase in surface area

due to the roughness of the interface with respect to a flat one [4]. In the main text we show $\Delta\Omega$ and the areas for $S_3$, here in Figure 5, we present the results for $S_1$ on the left and $S_2$ on the right. Here we present in panel **(a)** $\Delta\Omega$ and $\Delta\mathcal{F}$. In panel **(b)** we show $\Delta\mathcal{F}$ on the axis at the left (in blue) and all the components of Equation (3) on the right (in black). Panel **(c)** is similar to **(b)** but we show only $\Delta\mathcal{F}$ in blue and $A^{\mathrm{B}}_{\mathrm{GL}}$ in black. The dashed vertical lines indicates the maxima in $\Delta\mathcal{F}$.

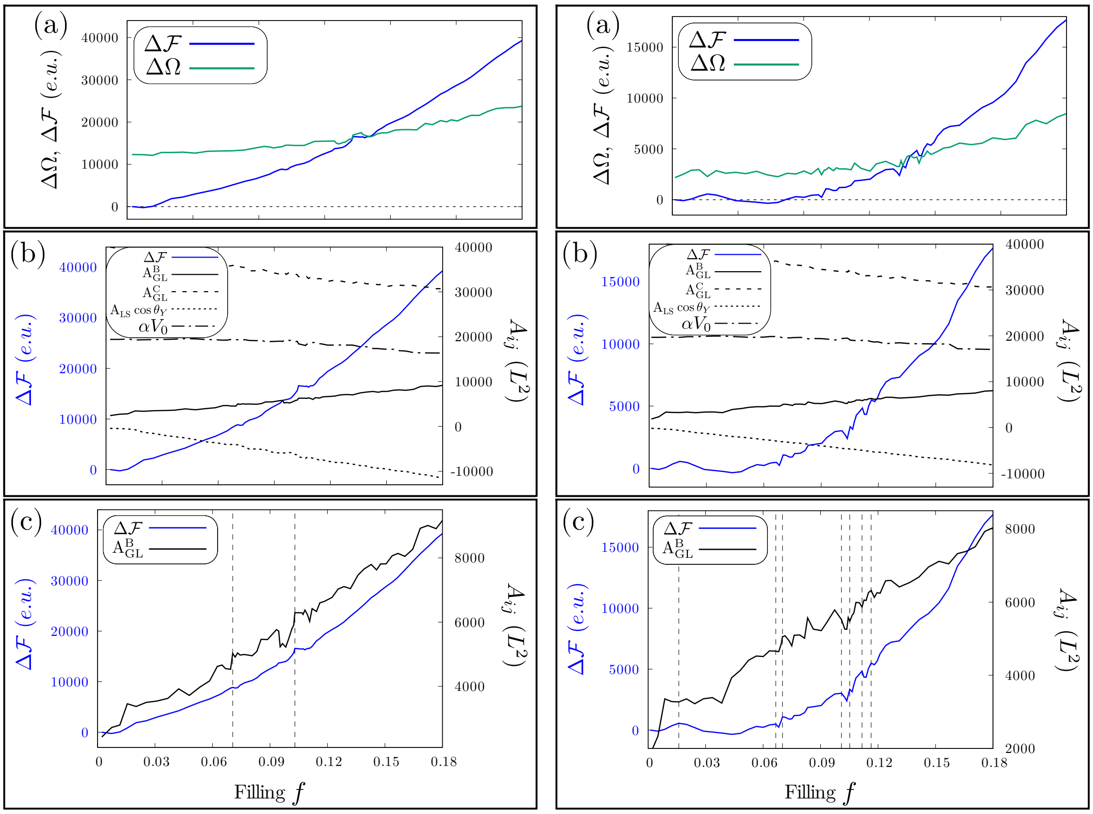


Figure 4: $\Delta\mathcal{F}$, $\Delta\Omega$ and areas as a function of $f$ for $S_1$ on the left and $S_2$ on the right. (a) Comparison of $\Delta\mathcal{F}$ and $\Delta\Omega$. (b) The free energy $\Delta\mathcal{F}$ is shown in blue (left axis) and the components of Equation (3) are shown in black (right axis): solid line is $A^{\mathrm{B}}_{\mathrm{GL}}$, dashed line is $A^{\mathrm{C}}_{\mathrm{GL}}$, dotted line is $A_{\mathrm{LS}}\cos\theta_{\mathrm{Y}}$, and dot-dashed line is $-\alpha V_0$. (c) Similar to (b) but with only $A^{\mathrm{B}}_{\mathrm{GL}}$. The red curve is a linear fit of $A^{\mathrm{B}}_{\mathrm{GL}}$ and the red vertical lines indicate the area variations discussed in the main text. Dashed lines denote the maxima of $\Delta\mathcal{F}$.

# References

[1] H. C. M. Fernandes, M. H. Vainstein, C. Brito, *Langmuir* **2015**, *31*, 27 7652.

[2] M. Silvestrini, C. Brito, *Langmuir* **2017**, *33*, 43 12535.

[3] C. Gavazzoni, M. Silvestrini, C. Brito, *J. Chem. Phys.* **2021**, *154*, 10 104704.

[4] R. Magno, V. Grieneisen, A. F. M. Marée, *BMC Biophys.* **2015**, *8*, 1 1.
